# Supplementary material for: Beyond Flatland: A Geometric Take on Matching Methods for Treatment Effect Estimation
Source: arXiv:2409.05459 source file (2025-05-05)
Supplement: Supplementary file 1 [file gplvm.tex]

\section{Learning latent Riemannian manifold using a GPLVM}\label{app:gplvm}

\subsection{Empirical Results}

\subsection{Discussion}

Main point, vanilla GPLVM does not preserve geometric structure. TODO: discuss and link to works trying to preserve geometry.
